# Supplementary material for: Thouless-Valatin Rotational Moment of Inertia from the Linear Response Theory
Source: arXiv:1709.08534 source file (2017-09-25)
Supplement: Supplementary file 1 [file Article2017suppl-v2.pdf]

# Thouless–Valatin Rotational Moment of Inertia from the Linear Response Theory Supplementary Material

Kristian Petrík
*Helsinki Institute of Physics, University of Helsinki, P.O. Box 64, FI-40014 Helsinki, Finland and Department of Physics, University of Jyvaskyla, P.O. Box 35, FI-40014 Jyvaskyla, Finland*

Markus Kortelainen
*Department of Physics, University of Jyvaskyla, P.O. Box 35, FI-40014 Jyvaskyla, Finland and Helsinki Institute of Physics, University of Helsinki, P.O. Box 64, FI-40014 Helsinki, Finland*

Here we wish to provide additional details and supplementary results about the main elements of our work. The following information should serve as an extension supporting the key conclusions obtained from the FAM–QRPA calculations of the Thouless–Valatin rotational moment of inertia. In particular, we present some specifics about the cranking calculations carried out with the HFB model and discuss additional results related to the induced isoscalar current density $\vec{j}_0$, and proton and neutron currents, $\vec{j}_\mathrm{p}$ and $\vec{j}_\mathrm{n}$, respectively.

## I. CRANKING CALCULATIONS

In Table I, we show the results of the Thouless–Valatin moment of inertia coming from the FAM–QRPA formalism as compared to the cranking model calculations. In both approaches, the SkM* Skyrme parametrization was employed with identical pairing strengths and we chose 12, 14 and 16 major oscillator shells in order to investigate possible effects of the model space size. These smaller, but sufficient numbers of shells were selected, mostly due to the computational costs of the cranking calculations. For the cranking approach, we used the HFODD computer program as the primary HFB solver. Cranking calculations were performed with different cranking frequencies and the listed moments of inertia were obtained from a quadratic extrapolation to zero cranking frequency.

We have obtained an excellent agreement between the two approaches with only minor differences. Moreover, the FAM–QRPA calculations were significantly faster, especially for the higher numbers of shells and were not dependent on the extrapolation to the zero frequency.

## II. INDUCED CURRENT DENSITY

In this section we discuss the flow characteristics of the induced isoscalar current density $\vec{j}_0$ and the separate contributions to this quantity from individual QRPA blocks (numbered by the projection quantum number $\Omega$). In addition, we study also the total proton and neutron currents. In the main text, we covered the results for the prolate deformed $^{166}$Er, hence, here we would like to examine also the oblate state of the same isotope. In order to investigate heavier systems and verify our conclusions, the heavy $^{240}$Pu nucleus is examined as well.

In Fig. 1, the neutron and proton induced currents of prolate $^{166}$Er are shown. The left panels (a)–(b) display the results for the volume pairing setup and the right panels (c)–(d) the case with the vanishing pairing. One can easily see the strong effect coming from the neutron flow, which contributes to the rotational component of the current. The magnitude is a natural consequence of the fact that $N > Z$, so neutrons contribute more to the rotational flow. However, qualitatively, there are only minor differences between neutrons and protons. When pairing is present, the irrotational component of the rotation is more dominant, which affects the final value of the Thouless–Valatin rotational inertia.

TABLE I. Thouless–Valatin rotational moment of inertia of deformed $^{166}$Er isotope, calculated in the FAM–QRPA and cranking model. Values are given in units of MeV$^{-1}$.

| Shells | 12 | 14 | 16 |
|---|---|---|---|
| FAM–QRPA | 34.866 | 35.398 | 34.511 |
| Cranking | 34.887 | 35.450 | 34.533 |

In Figs. 2 and 3, we can see the total induced current (a) and its separate contributions per QRPA blocks (b)–(e) of oblate $^{166}$Er configuration for the cases with the volume pairing and with no pairing, respectively. See the main text for the explanation about the QRPA blocks.

In Fig. 4, these results are shown on the level of separate neutron and proton flows. The same discussion holds as previously, pairing correlations lead to the suppression of the rotational components of the motion and enhance the irrotational character of the current. We again observe a strong effect coming from the QRPA blocks 6 and 7 as it was in the case of the prolate $^{166}$Er in our article.

In Figs. 5 and 6, we present the results for the heavy deformed $^{240}$Pu. The total induced current (a) is indicated along with the per QRPA block contributions (b)–(e). In Fig. 7, the proton and neutron currents are given with and without pairing present.

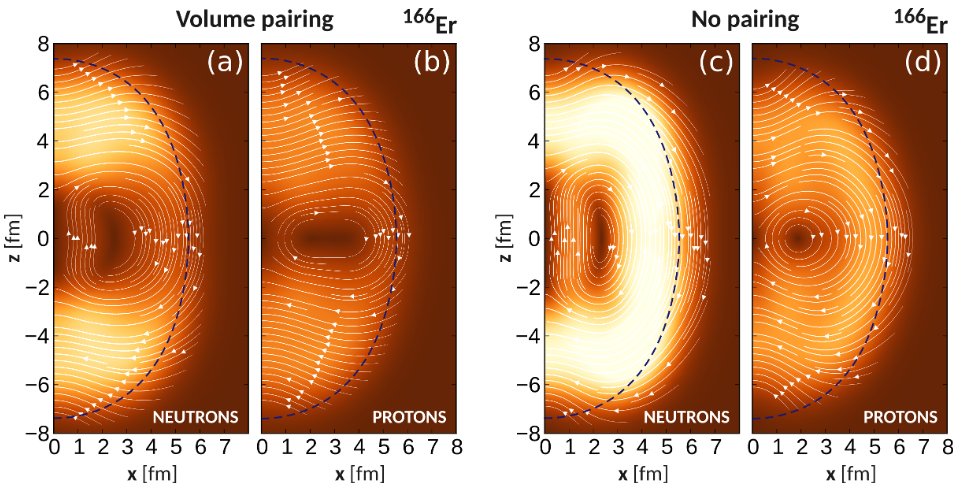


FIG. 1. Neutron and proton induced current densities, $\vec{j}_{\rm n}$ and $\vec{j}_{\rm p}$, respectively, of prolate $^{166}$Er are shown in the $x$–$z$ plane. The lighter color indicates a larger amplitude. Panels (a) and (b) display results for the volume pairing setup and panels (c) and (d) the results without pairing.

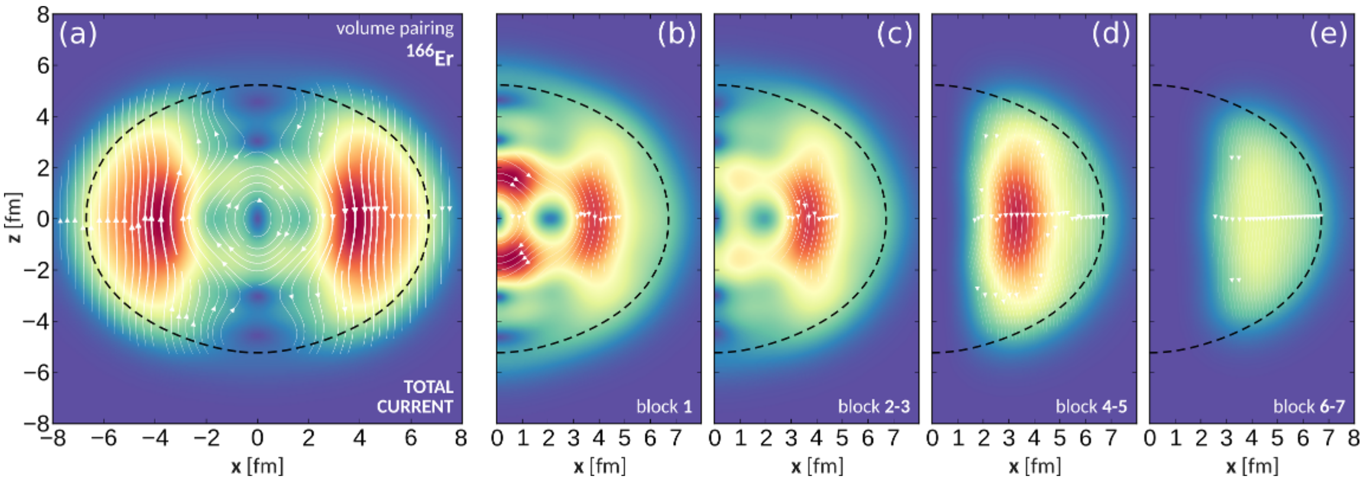


FIG. 2. The flow (lines with arrows) of the induced isoscalar current density $\vec{j}_0$ and its amplitude (color and line thickness) for the oblate $^{166}$Er with the volume pairing setup are shown in the $x$–$z$ plane. The left panel (a) displays the total induced current and the right panels (b)–(e) the partial contributions to it as given by the specific QRPA blocks. The black dashed contour line indicates the nuclear surface at matter density of $\rho_0 = 0.08\,\mathrm{fm}^{-3}$.

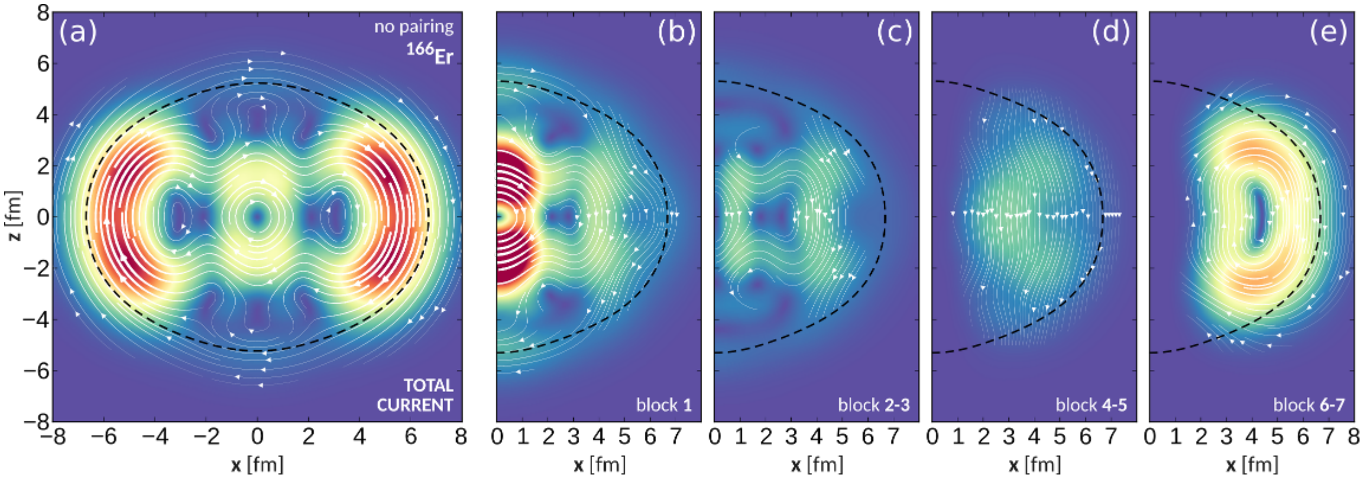


FIG. 3. The same as Fig. 2, but without pairing.

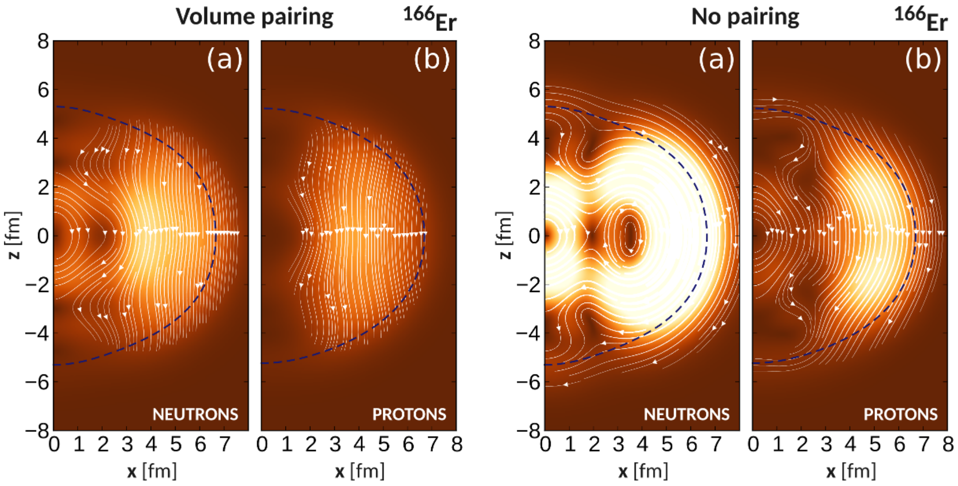


FIG. 4. The same as Fig. 1, but for the oblate configuration of $^{166}$Er.

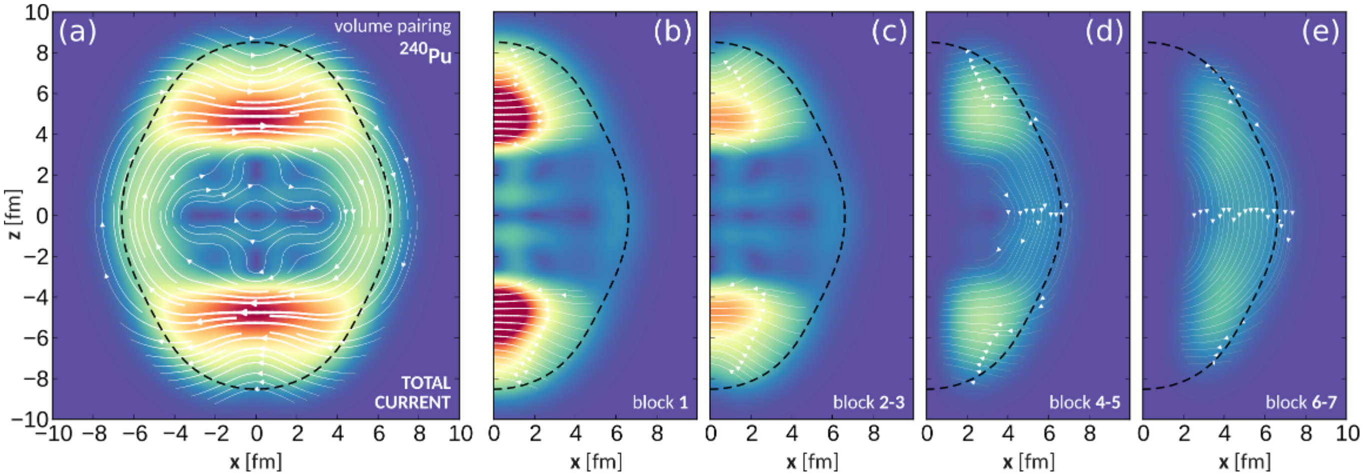


FIG. 5. The same as Fig. 2 but for $^{240}$Pu with volume pairing.

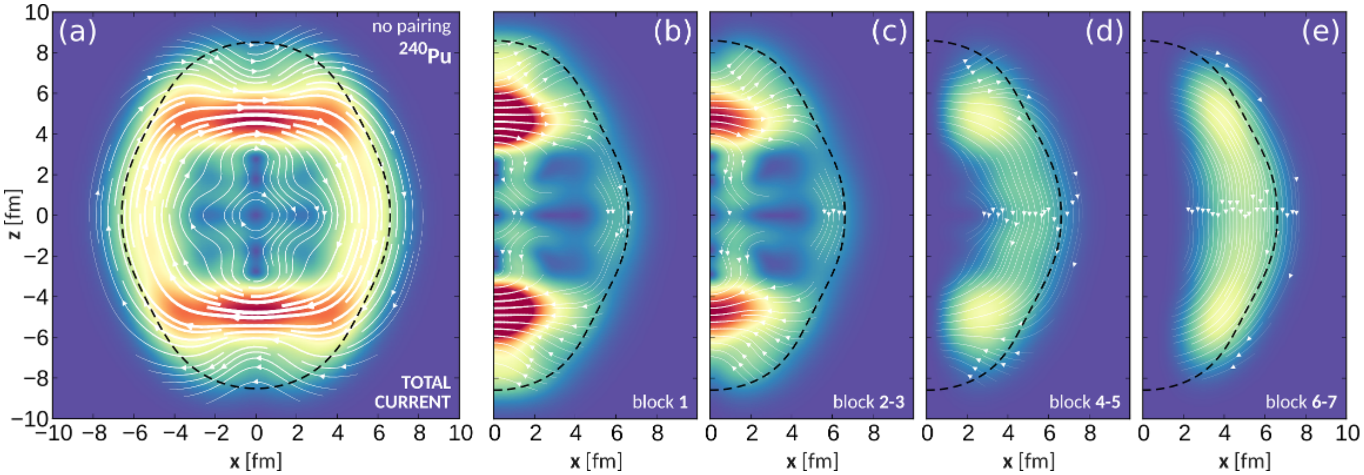


FIG. 6. The same as Fig. 2 but for $^{240}$Pu without pairing.

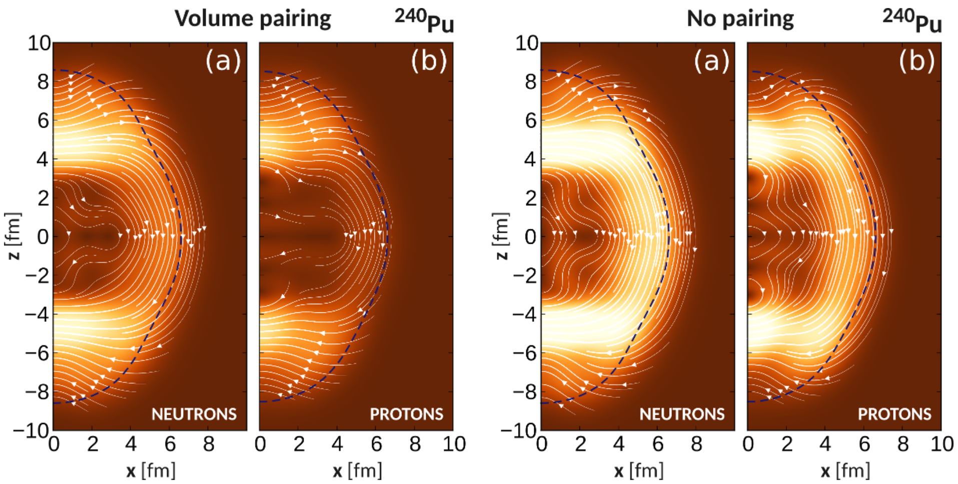


FIG. 7. The same as Fig. 1, but for $^{240}$Pu.
